# Supplementary material for: Estimating conditional means under missingness-not-at-random with incomplete auxiliary variables
Source: arXiv:2611.26891 source file (2026-11-19)
Supplement: Supplementary file 1 [file preamble_appendix.tex]

\usepackage[T1]{fontenc} %
\usepackage{microtype} %
\usepackage[singlespacing]{setspace}

\usepackage[margin=1in]{geometry}
\usepackage{lineno}

\usepackage{multicol} %
\usepackage[hang, small,labelfont=bf,up,textfont=it,up]{caption} %
\usepackage{booktabs} %
\usepackage{multirow}
\usepackage{siunitx}
\usepackage{float} %
\usepackage{lettrine} %
\usepackage{outlines}
\usepackage{sansmath}
\usepackage{thmtools} %

\usepackage[hyphens]{url}

\usepackage[american]{babel}
\usepackage[style=american]{csquotes}
\usepackage[autocite=superscript,sorting=none,sortcites=true]{biblatex}
\addbibresource{refs.bib}
\renewbibmacro{in:}{}
\DeclareNameAlias{default}{labelname}

\usepackage[svgnames]{xcolor}
\usepackage{listings}
\usepackage{comment, mdframed, makecell}

\setlength\parindent{0pt}
\setlength{\parskip}{1em}  %

\lstset{language=R,
    basicstyle=\small\ttfamily,
    commentstyle=\color{Red},
    columns=fullflexible,
  frame=single,
  breaklines=true }

\newcommand{\rc}[1][]{\textsuperscript{\orange{(cite)}} }

\usepackage{amsmath,amsfonts,amsthm, textcomp, bm, bbm} %

\makeatletter
\renewcommand*\env@matrix[1][\arraystretch]{%
  \edef\arraystretch{#1}%
  \hskip -\arraycolsep
  \let\@ifnextchar\new@ifnextchar
  \array{*\c@MaxMatrixCols c}}
\makeatother

\usepackage{array}
\newcolumntype{L}[1]{>{\raggedright\let\newline\\\arraybackslash\hspace{0pt}}m{#1}}
\newcolumntype{C}[1]{>{\centering\let\newline\\\arraybackslash\hspace{0pt}}m{#1}}
\newcolumntype{R}[1]{>{\raggedleft\let\newline\\\arraybackslash\hspace{0pt}}m{#1}}

\usepackage{graphicx}
\usepackage{float}
\usepackage{booktabs} %
 \usepackage{ amssymb }
 
 \usepackage{todonotes}
 \usepackage{dsfont} %

\usepackage{titlesec} %
\titleformat{\section}[block]{\large\bfseries}{\thesection.}{1em}{} %
\titleformat{\subsection}[block]{\large}{\thesubsection.}{1em}{} %

\usepackage{fancyhdr} %
\pagestyle{fancy} %
\fancyhead{} %
\fancyfoot{} %
\fancyhead[C]{Supplement} %
\fancyfoot[RO,LE]{\thepage} %

\usepackage{graphicx}

\usepackage{xcolor}
\usepackage{color}
\usepackage{soul}
\soulregister\ref7 %

\renewcommand\theequation{S\arabic{equation}}
\setcounter{equation}{0}

\renewcommand{\thetable}{S\arabic{table}}
\renewcommand{\thefigure}{S\arabic{figure}}

\definecolor{junglegreen}{rgb}{0.16, 0.67, 0.53}
\definecolor{lav}{rgb}{0.71, 0.49, 0.86}
\newcommand{\red}[1]{\textcolor{red}{#1}}
\newcommand{\orange}[1]{\textcolor{orange}{#1}}
\newcommand{\blue}[1]{\textcolor{blue}{#1}}
\newcommand{\black}[1]{\textcolor{black}{#1}}
\newcommand{\pink}[1]{\textcolor{pink}{#1}}
\newcommand{\lav}[1]{\textcolor{lav}{#1}}
\newcommand{\green}[1]{\textcolor{junglegreen}{#1}}
\newcommand{\redf}[1]{\footnote{\textcolor{red}{#1}}}
\newcommand{\bluef}[1]{\footnote{\textcolor{blue}{#1}}}
\newcommand{\greenf}[1]{\footnote{\textcolor{junglegreen}{#1}}}
\newcommand{\orangef}[1]{\footnote{\textcolor{orange}{#1}}}

\usepackage{pgfplotstable}
\usepackage{csvsimple}
\usepackage{siunitx}

\newcommand{\datafoldername}{R_objects}

\newcommand{\rlgetvalue}[4]{\csvreader[filter strcmp={\mykey}{#3},
             late after line = {{,}\ }, late after last line = {{}}]
            {\datafoldername/#1}{#2=\mykey,#4=\myvalue}{\myvalue}}

\newcommand{\rlgetvariable}[1]{\csvreader[]{\datafoldername/myvars.csv}{#1=\myvar}{\myvar}\xspace}

\newcommand{\rlnum}[2]{\num[output-decimal-marker={.},
                             exponent-product = \cdot,
                             round-mode=places,
                             round-precision=#2,
                             group-digits=false]{#1}}

\newcommand{\rlnumsci}[2]{\num[output-decimal-marker={.},
                          scientific-notation = true,
                             exponent-product = \cdot,
                             round-mode=places,
                             round-precision=#2,
                             group-digits=false]{#1}}

\newcommand{\rlgetnum}[5]{\csvreader[filter strcmp={\mykey}{#3},
             late after line = {{,}\ }, late after last line = {{}}]
            {\datafoldername/#1}{#2=\mykey,#4=\myvalue}{\rlnum{\myvalue}{#5}}}

\newcommand{\rlgetnumsci}[5]{\csvreader[filter strcmp={\mykey}{#3},
             late after line = {{,}\ }, late after last line = {{}}]
            {\datafoldername/#1}{#2=\mykey,#4=\myvalue}{\rlnumsci{\myvalue}{#5}}}

\usepackage{algorithm, algorithmic} %
\renewcommand{\algorithmicrequire}{\textbf{Input:}}
\renewcommand{\algorithmicensure}{\textbf{Output:}}

\usepackage{tikz}
\usetikzlibrary{shapes,decorations,arrows,calc,arrows.meta,fit,positioning}
\tikzset{
    -Latex,auto,node distance =1 cm and 1 cm,semithick,
    state/.style ={ellipse, draw, minimum width = 0.7 cm},
    point/.style = {circle, draw, inner sep=0.04cm,fill,node contents={}},
    bidirected/.style={Latex-Latex,dashed},
    el/.style = {inner sep=2pt, align=left, sloped}
}

\usetikzlibrary{arrows,shapes.arrows,shapes.geometric,
shapes.multipart,decorations.pathmorphing,positioning,
swigs}

 

\renewcommand{\thefootnote}{\textit{\alph{footnote}}}

\newtheoremstyle{spaceythm}
  {2\topsep} %
  {2\topsep} %
  {} %
  {} %
  {\bfseries} %
  {.} %
  {.5em} %
  {} %

\theoremstyle{spaceythm}
\newtheorem{theorem}{Theorem}
\newtheorem{assumption}{Assumption}
\newtheorem{remark}{Remark}
\newtheorem{proposition}{Proposition}
\newtheorem{lemma}{Lemma}
\newtheorem{corollary}{Corollary}
\newtheorem{definition}{Definition}

\renewcommand\theassumption{A\arabic{assumption}}

\newtheorem{slemma}{Lemma}
\renewcommand{\theslemma}{S\arabic{slemma}}
\newtheorem{sproposition}{Proposition}
\renewcommand{\thesproposition}{S\arabic{sproposition}}
\newtheorem{scorollary}{Corollary}
\renewcommand{\thescorollary}{S\arabic{scorollary}}
\newtheorem{sdefinition}{Definition}
\renewcommand{\thesdefinition}{S\arabic{sdefinition}}
\renewcommand{\thealgorithm}{S\arabic{algorithm}}
\newtheorem{sremark}{Remark}
\renewcommand{\thesdefinition}{S\arabic{sdefinition}}

\newtheorem{spaceythm}[theorem]{\thistheoremname}

\newenvironment{namedthm}[1]
  {\renewcommand{\thistheoremname}{#1}%
   \begin{spaceythm}}
  {\end{spaceythm}}

  
\newtheorem*{spaceythm*}{\thistheoremname}
\makeatletter
\newcounter{namedthmctr} %
\newenvironment{namedthm*}[1]
  {%
    \renewcommand{\thistheoremname}{#1}%
    \def\thm@name{#1}%
    \refstepcounter{namedthmctr}%
    \let\thm@oldlabel\label
    \renewcommand{\label}[1]{%
      \begingroup
      \protected@edef\@currentlabelname{\thm@name}%
      \thm@oldlabel{##1}%
      \endgroup
    }%
    \begin{spaceythm*}%
  }
  {%
    \end{spaceythm*}%
    \let\label\thm@oldlabel
  }
\makeatother

\theoremstyle{named}
\newtheorem*{namedtheorem}{Theorem}

\setcounter{lemma}{0}

\newcounter{scounter}

\makeatletter
\newtheoremstyle{suppstyle}%
  {2\topsep}{2\topsep}              %
  {\itshape}        %
  {}                %
  {\bfseries}       %
  {}                %
  {0.5em}           %
  {\thmname{#1}\thmnumber{ #2}} %
\makeatother

\theoremstyle{suppstyle}

\usepackage{xcolor}
\newcommand{\ilya}[1]{{\color{red!70!blue} #1}}
\usepackage[normalem]{ulem} %
\newcommand{\stkout}[1]{\ifmmode\text{\sout{\ensuremath{#1}}}\else\sout{#1}\fi}

\newtheorem{thm}{Theorem}[section] %
\theoremstyle{plain} %
\newcommand{\thistheoremname}{}

\usepackage[bottom]{footmisc}

\makeatletter
\renewcommand{\boxed}[1]{\text{\fboxsep=.2em\fbox{\m@th$\displaystyle#1$}}}
\makeatother

\newcommand{\remindcite}[1][]{ \textsuperscript{\orange{(cite)}} }

\newcommand{\hlcyan}[1]{{\sethlcolor{cyan}\hl{#1}}}

\newif\ifshowSecrets

\ifshowSecrets
  \newcommand{\hlDef}[1]{\hl{#1}}
  \newcommand{\hlDefMath}[1]{ \text{ \hl{ $#1$ } } }
  \newcommand{\secretf}[1]{\footnote{\textcolor{junglegreen}{#1}}}
  \newcommand{\secreti}[1]{\textcolor{junglegreen}{#1}}
  \newcommand{\assume}[1]{\textcolor{blue}{\uwave{#1}}}
  \newenvironment{secret}{\color{junglegreen}}{}
\else
  \newcommand{\hlDef}[1]{#1}
  \newcommand{\hlDefMath}[1]{#1}
  \newcommand{\secretf}[1]{}
  \newcommand{\secreti}[1]{}
  \newcommand{\assume}[1]{#1}
  \excludecomment{secret}
\fi

\usepackage{xr-hyper}   %

\usepackage{subcaption}

\fancyhead[C]{Supplement} %

\title{\vspace{-15mm}\fontsize{18pt}{19pt}\selectfont\textbf{Full Title}} %
