# Supplementary material for: Estimating conditional means under missingness-not-at-random with incomplete auxiliary variables
Source: arXiv:2611.26891 source file (2026-11-19)
Supplement: Supplementary file 3 [file xr_supp_labels.tex]

\makeatletter
\newlabel{supp-tb:results_index}{{S1}{2}{}{}{}}
\newlabel{supp-fig:proof_dependency_flowchart}{{S1}{3}{}{}{}}
\newlabel{supp-sec:DAGs}{{1.1}{3}{}{}{}}
\newlabel{supp-sec:review_assumptions}{{1.2}{5}{}{}{}}
\newlabel{supp-ass:boring_assumptions}{{A0}{5}{}{}{}}
\newlabel{supp-ass:partial_faithfulness}{{A0(i)}{5}{}{}{}}
\newlabel{supp-ass:no_determinism}{{A0(ii)}{5}{}{}{}}
\newlabel{supp-ass:cc_positivity}{{A0(iii)}{5}{}{}{}}
\newlabel{supp-ass:no_cancellations}{{A0(iv)}{5}{}{}{}}
\newlabel{supp-ass:positivity}{{A1}{5}{}{}{}}
\newlabel{supp-ass:no_csi}{{A2}{5}{}{}{}}
\newlabel{supp-def:perfect_cancellations_sums_fns}{{S1}{6}{}{}{}}
\newlabel{supp-def:pattern_regularity}{{S2}{6}{}{}{}}
\newlabel{supp-lm:pattern_regularity}{{S1}{6}{}{}{}}
\newlabel{supp-eq:interm2}{{S1}{6}{}{}{}}
\newlabel{supp-prop:wneg_cant_fix_mnar}{{1}{7}{}{}{}}
\newlabel{supp-rm:Omega_function_vs_rv}{{1}{7}{}{}{}}
\newlabel{supp-sec:H}{{2.1}{8}{}{}{}}
\newlabel{supp-def:functionally_determining_set}{{S3}{8}{}{}{}}
\newlabel{supp-lm:unique_mfds}{{S2}{8}{}{}{}}
\newlabel{supp-coro:mfds_sums}{{S1}{9}{}{}{}}
\newlabel{supp-prop:H_characterization}{{S1}{9}{}{}{}}
\newlabel{supp-eq:barbara}{{S2}{10}{}{}{}}
\newlabel{supp-eq:jack}{{S3}{10}{}{}{}}
\newlabel{supp-sec:wcc_conditions}{{2.2}{11}{}{}{}}
\newlabel{supp-lm:empty_interior_solution_set}{{S3}{11}{}{}{}}
\newlabel{supp-thm:wcc_conditions}{{1}{12}{}{}{}}
\newlabel{supp-eq:wtd_est_eqs}{{S4}{12}{}{}{}}
\newlabel{supp-eq:38309}{{S5}{13}{}{}{}}
\newlabel{supp-coro:wcc_suff_conditions}{{1}{13}{}{}{}}
\newlabel{supp-lm:Y_R_plus_MNAR_muMAR_incorrect}{{S4}{14}{}{}{}}
\newlabel{supp-eq:pattern_dependence}{{S6}{14}{}{}{}}
\newlabel{supp-eq:pmar_sum}{{S7}{15}{}{}{}}
\newlabel{supp-rm:averaging_cancellations}{{2}{15}{}{}{}}
\newlabel{supp-thm:IPW_with_incomplete_Y}{{2}{15}{}{}{}}
\newlabel{supp-thm:mia_conditions}{{3}{16}{}{}{}}
\newlabel{supp-lm:C1_MIA_numerator}{{S5}{17}{}{}{}}
\newlabel{supp-lm:C2_MIA_Y_R_path}{{S6}{17}{}{}{}}
\newlabel{supp-fig:witnessing_path_Wneg_figure}{{S2}{19}{}{}{}}
\newlabel{supp-lm:Omega_FD_on_Y}{{S7}{20}{}{}{}}
\newlabel{supp-thm:IPW_with_Wneg}{{4}{21}{}{}{}}
\newlabel{supp-sec:domination_thm}{{2.6}{21}{}{}{}}
\newlabel{supp-thm:dominating_cases_af4}{{5}{21}{}{}{}}
\newlabel{supp-sec:discrete_X_aipw_tmle}{{3}{22}{}{}{}}
\newlabel{supp-eq:mia_eif}{{S10}{22}{}{}{}}
\newlabel{supp-eq:mia_eif_est_eqs}{{S11}{23}{}{}{}}
\newlabel{supp-eq:muhatMIAaipw}{{S12}{23}{}{}{}}
\newlabel{supp-sec:estimation_general_case}{{4}{23}{}{}{}}
\newlabel{supp-eq:CATE.definition.equivalent}{{S13}{24}{}{}{}}
\newlabel{supp-eq:CATE.loss}{{S14}{24}{}{}{}}
\newlabel{supp-eq:equivalent.loss.fn}{{S15}{24}{}{}{}}
\newlabel{supp-eq:AIPW1}{{S16}{24}{}{}{}}
\newlabel{supp-eq:AIPW2}{{S17}{25}{}{}{}}
\newlabel{supp-eq:recognise}{{S18}{25}{}{}{}}
\newlabel{supp-eq:Shaunequation}{{S19}{25}{}{}{}}
\newlabel{supp-sect:Shaunproof1}{{4.3}{27}{}{}{}}
\newlabel{supp-eq:expand.loss}{{S20}{27}{}{}{}}
\newlabel{supp-sect:Shaunproof2}{{4.4}{27}{}{}{}}
\newlabel{supp-sec:nice_estimator}{{5}{28}{}{}{}}
\newlabel{supp-alg:MIA}{{S1}{29}{}{}{}}
\newlabel{supp-sec:applied}{{6}{29}{}{}{}}
\newlabel{supp-tb:applied_var_defns}{{S2}{30}{}{}{}}
\newlabel{supp-fig:missing_pattern}{{S3}{31}{}{}{}}
\newlabel{supp-tb:baseline_characteristics_2}{{S3}{31}{}{}{}}
\newlabel{supp-fig:applied_forest_plot_check}{{S4}{32}{}{}{}}
\newlabel{supp-fig:applied_dharma_mia_ice_model_2}{{S5}{33}{}{}{}}
\newlabel{supp-fig:applied_dharma_mia_ice_model_3}{{S6}{33}{}{}{}}
\newlabel{supp-fig:applied_dharma_mia_ice_model_4}{{S7}{34}{}{}{}}
\newlabel{supp-fig:applied_mice_model_1_convergence}{{S8}{34}{}{}{}}
\newlabel{supp-fig:applied_mice_model_2_convergence}{{S9}{34}{}{}{}}
\newlabel{supp-fig:applied_mice_model_3_convergence}{{S10}{35}{}{}{}}
\newlabel{supp-fig:applied_mice_model_4_convergence}{{S11}{35}{}{}{}}
\newlabel{supp-fig:applied_mice_model_1_distribution_id}{{S12}{35}{}{}{}}
\newlabel{supp-fig:applied_mice_model_2_distribution_id}{{S13}{36}{}{}{}}
\newlabel{supp-fig:applied_mice_model_2_distribution_occ}{{S14}{36}{}{}{}}
\newlabel{supp-fig:applied_mice_model_3_distribution_id}{{S15}{37}{}{}{}}
\newlabel{supp-fig:applied_mice_model_4_distribution_id}{{S16}{37}{}{}{}}
\newlabel{supp-fig:applied_mice_model_4_distribution_occ}{{S17}{38}{}{}{}}
\newlabel{supp-sec:sim_study}{{7}{39}{}{}{}}
\newlabel{supp-sec:sims_univariate_W}{{7.1}{39}{}{}{}}
\newlabel{supp-tb:sim_n200_wdim1}{{S4}{42}{}{}{}}
\newlabel{supp-tb:sim_n500_wdim1}{{S5}{43}{}{}{}}
\newlabel{supp-tb:sim_n1000_wdim1}{{S6}{44}{}{}{}}
\newlabel{supp-tb:sim_n2000_wdim1}{{S7}{45}{}{}{}}
\newlabel{supp-tb:sim_n5000_wdim1}{{S8}{46}{}{}{}}
\newlabel{supp-tb:sim_n10000_wdim1}{{S9}{47}{}{}{}}
\newlabel{supp-sec:sims_highdim_W}{{7.2}{47}{}{}{}}
\newlabel{supp-tb:sim_n1000_wdim10}{{S10}{49}{}{}{}}
\newlabel{supp-tb:sim_n2000_wdim10}{{S11}{50}{}{}{}}
\newlabel{supp-tb:sim_n5000_wdim10}{{S12}{51}{}{}{}}
\newlabel{supp-tb:sim_n10000_wdim10}{{S13}{52}{}{}{}}
\newlabel{supp-sec:sims_assumptions_violated}{{7.3}{52}{}{}{}}
\newlabel{supp-tb:sim3_N200}{{S14}{56}{}{}{}}
\newlabel{supp-tb:sim3_N500}{{S15}{57}{}{}{}}
\newlabel{supp-tb:sim3_N1000}{{S16}{58}{}{}{}}
\newlabel{supp-tb:sim3_N5000}{{S17}{59}{}{}{}}
\newlabel{supp-tb:sim3_N10000}{{S18}{60}{}{}{}}
\makeatother
